# Supplementary material for: VR-Goggles for Robots: Real-to-sim Domain Adaptation for Visual Control
Source: arXiv:1802.00265 source file (2019-01-16)
Supplement: Supplementary file 1 [file appendix2.tex]

\subsection{Comparing Policy Transfer Methods: Simulated Indoor Navigation}
\label{sec:experiments-transfer-comparison}

\begin{figure}[!b]
    \centering
        \includegraphics[width=0.8\columnwidth]{imgs/domain_randomization}
    % \vspace{-0.1in}
    \caption{
8 different sets of textures of the 8 workers for training \textit{Multi-Domain}
%our A3C variant of \textit{Randomization}
(Sec. \ref{sec:experiments-transfer-comparison}).
    }
    \label{fig:domain-randomization}
\end{figure}

\begin{figure*}[!t]
    \hspace{0.3in}\includegraphics[width=.9\textwidth]{imgs/transfer_compare}
    \vspace{-0.1in}
    \caption{
Average episode lengths in evaluation during training,
comparing policy transfer procedures of \textit{From-Scratch}, \textit{Multi-Domain} and \textit{Progressive}.
We show median-filtered curves in line with \cite{rusu2016sim}.
An adapting phase is necessary for \textit{Progressive} in each new environment; while for our \textit{real-to-sim} approach,
\textit{From-Scratch} is all the policy training needed.
}
    \label{fig:transfer-compare}
\end{figure*}

To illustrate the difference between the policy transfer pipelines
of our proposed \textit{real-to-sim} approach
and several representative \textit{sim-to-real} approaches
%discussed in Sec. \ref{sec:related-da-drl},
we conduct a direct comparison in a simulated indoor navigation experiment.

We build an indoor office environment in \textit{Gazebo} \cite{koenig2004design}.
With two different sets of textures,
we render two environments:
\textit{\textbf{Sim-Env}} and
\textit{\textbf{"Real"-Env}}, shown on the left of Fig. \ref{fig:transfer-compare}.
We train agents to learn navigation policies
to accomplish the task of navigating to chairs based purely on its front-facing color camera readings; the agent obtained a reward of $-0.005$ for a step cost, $-0.05$ for collision, and $1$ for reaching the target.
We illustrate the procedures of the following approaches to transfer policies learned in \textit{Sim-Env} to \textit{"Real"-Env},
and show the average steps obtained by the agents in evaluation during training in Fig. \ref{fig:transfer-compare}:

(1) \textit{\textbf{From-Scratch}} \cite{mnih2016asynchronous}:
Canonical A3C trained from scratch on \textit{Sim-Env}.
We execute 8 training processes and 1 evaluation process,
each with their own copy of \textit{Sim-Env}.
We note here that this is all the policy training required for our \textit{real-to-sim} approach,
as no fine-tuning or retraining of the policy is needed for deploying it in real-world scenes;
also, since our approach decouples the policy training and the domain adaptation,
the adaptation networks can be trained in parallel with the policy training.
This is also the policy training procedure for several sim-to-real approaches
\cite{bousmalis2017using,stein2018genesis},
except that an additional adaptation step has to be added for each of the training frames;
also, for each visually different real-world scene,
this line of approaches needs to go through another complete policy training procedure.
(2) \textit{\textbf{Multi-Domain}} (inspired by \cite{Sadeghi2017cadrl, tobin2017domain}):
Our A3C variant of the \textit{domain randomization} approach.
The key concept of \textit{domain randomization} \cite{Sadeghi2017cadrl,tobin2017domain} is randomizing the textures, viewing angles, etc. of objects during the training in simulation,
such that when deploying the trained model in real-world scenarios,
the modality of the real-world objects could just be naturally dealt with as another variation.
Here we adopt the same basic idea but implement it under the constraints of our simulator
(changing the texture for each frame is not as straightforward in \textit{Gazebo}).
In detail,
each of the 8 A3C workers renders its environment with its own set of textures.
All 8 sets of textures for the various objects in the environment are shown in Fig. \ref{fig:domain-randomization}.
The evaluation during training uses \textit{Sim-Env} as its environment.
We note here that this is all the policy training required for the \textit{Multi-Domain} approach,
since once converged, the agent is expected to be directly deployable in real-world environments.
Unfortunately, for our considered task and setup,
our A3C variant of the approach does not manage to learn useful policies,
as is shown by the green dashed line in Fig. \ref{fig:transfer-compare}
(we trained it for 8 times the iterations shown but still it fails to converge).
We suspect that our variant of randomizing textures might have imposed challenges for our RL task where informative reward signals are sparse. We suspect that more workers with more sets of textures could lead to improved performance. However, with relatively limited computing resources and with simulators where there is no relatively efficient solutions for randomizing the textures of objects at each frame, the \textit{Multi-Domain} method does not learn useful policies.
%may not enough for this task.
%Considering the higher cost to design randomized environments in \textit{Gazebo},
% It shows that domain randomization may not be applicable in simulated environments like \textit{Gazebo} which costs too many efforts for texture randomization.
% We suspect that different from the supervised learning task presented by \cite{tobin2017domain}
% where the supervision signal is strong and direct,
% with the sparse and delayed reward signals in our reinforcement learning task,
% the randomization might have imposed too many challenges for learning useful policies.
(3) \textit{\textbf{Progressive}} \cite{rusu2016sim}:
\textit{Progressive Nets} for transferring the policy of \textit{From-Scratch} on \textit{Sim-Env} to \textit{"Real"-Env}.
As described in \cite{rusu2016sim},
a second column is added after the first column is trained (the \textit{From-Scratch} policy on \textit{Sim-Env}).
% \footnote{We follow the same parameter initialization strategy as in \cite{rusu2016sim} for the output layers and the connection layers
% to guarantee that the initial policy output of the agent is identical to the first column.
% Observing that the simulation and real-world environments presented in \cite{rusu2016sim} are relateively more visually similar than \textit{Sim-Env} and \textit{"Real"-Env1},
% we additionally conduct experiments where we do not incorporate the above parameter initialization strategy,
% as we suspect that a random initialization might be more beneficial for transfer scenarios where
% two environments are more visually different.
% We found out that both the identical and the random initialization works,
% with the former converging faster.
% So we only report the experiments with the identical initialization,
% shown in the blue line in Fig. \ref{fig:transfer-compare}.}.
We note that for this approach,
although the adaptation of the policy in new environments is significantly accelerated compared to training from scratch,
the overall policy training needed contains both the initial training
(the yellow block),
and an adapting phase (the cyan blocks) in case we want to deploy
the agent in new environments.%,
% e.g., \textit{Real-Env2}, \textit{Real-Env3}.

% Having illustrated the advantage of our method in the \textit{policy training} part,
% we continue to compare different approaches of implementing the \textit{domain adaptation} part for our \textit{real-to-sim} approach.

% \hl{How long time do we need to train an domain adaptation model to deploy our policy in "Real"-Env?}

% We believe the experiments and discussions above validate our setout objective
% \hl{of proposing a lightweight, flexible and efficient solution} for dealing with the \textit{reality gap}.
%
% Having illustrated the policy training part, in the next section, we compare different approaches of implementing the \textit{domain adaptation} part for our \textit{real-to-sim} approach.

Further implementation details for \textit{Progressive}:
We follow the same parameter initialization strategy as in \cite{rusu2016sim} for the output layers and the connection layers
to guarantee that the initial policy output of the agent is identical to the first column.
Observing that the simulation and real-world environments presented in \cite{rusu2016sim} are relatively more visually similar than \textit{Sim-Env} and \textit{Real-Env},
we additionally conduct experiments where we do not incorporate the above parameter initialization strategy,
as we suspect that a random initialization might be more beneficial for transfer scenarios where
two environments are more visually different.
We found out that both the identical and the random initialization works,
with the former converging faster.
So we only report the experiments with the identical initialization,
shown in the blue line in Fig. \ref{fig:transfer-compare}.
