# Supplementary material for: VR-Goggles for Robots: Real-to-sim Domain Adaptation for Visual Control
Source: arXiv:1802.00265 source file (2019-01-16)
Supplement: Supplementary file 2 [file appendix3.tex]

\subsection{Comparing Domain Adaptation Methods: Additional Materials}
\label{apd:outdoor-da}

We additionally validate the \textit{shift loss} in the field of \textit{domain adaptation} in \textit{outdoor} urban street scenarios (where we collect synthetic domain images $s \sim p_{\text{sim}}$ from the \textit{CARLA} simulator \cite{dosovitskiy2017carla}, and realistic domain images $r \sim p_{\text{real}}$ from the \textit{RobotCar} dataset \cite{RobotCarDatasetIJRR}). We compare the following three setups:
\textit{\textbf{CyCADA}} \cite{hoffman2017cycada}: \textit{CycleGAN} with semantic constraints, trained on single frames;
\textit{\textbf{CyCADA+flow}}: \textit{CyCADA} with temporal constraints (\cite{huang2017real}), trained on sequential frames;
\textit{\textbf{Ours}}: \textit{CyCADA} with \textit{shift loss}, trained on single frames; we refer to this as the \textit{VR-Goggles}.

We pretrain the segmentation network $f_\mathcal{S}$ using \textit{Deeplab} \cite{chen2016deeplab}.
It is worth mentioning that the original \textit{CyCADA} paper did not use the semantic constraint in their experiments due to memory issues.
We are able to incorporate semantic loss calculation, by cropping the input in each iteration.

In Fig. \ref{fig:carla2robotcar}, we show a comparison of the subsequent frames generated by the three approaches. Our method again achieves the highest consistency and eliminates more artifacts due to the smoothness of the learned model.

\begin{figure}[!h]
    \centering
        \includegraphics[width=\columnwidth]{imgs/domain_adapt/carla2robotcar}
    \vspace{-0.01in}
    \caption{
    Comparison of the translated images for sequential input frames for the different approaches.
    $\nth{1}$ \textit{row}: two subsequent input frames from the realistic domain, with several representative images from the simulated domain shown in between;
    $\nth{2}\sim\nth{4}$ \textit{row}: outputs from \textit{CyCADA}, \textit{CyCADA+flow} and \textit{Ours}.
    Our method is able to output consistent subsequent frames and eliminate artifacts.
    We adjust the brightness of some zoom-ins for visualization purposes.}
    \label{fig:carla2robotcar}
\end{figure}

An additional implementation detail for all our \textit{domain adaptation} experiments:
As a naive random crop would highly likely lead to semantic permutations,
we crop inputs of the two domains in the same training iteration from the same random position,
and our empirical results show that this greatly stabilizes the adaptation.
