# Supplementary material for: VR-Goggles for Robots: Real-to-sim Domain Adaptation for Visual Control
Source: arXiv:1802.00265 source file (2019-01-16)
Supplement: Supplementary file 3 [file appendix4.tex]

\subsection{Detils for artistic style transfer and temporal error map}
For the sequence artistic style transfer, implementation wise, we use the pretrained \textit{VGG-19} as the loss network, \textit{relu}2\_2 as the content layer, \textit{relu}1\_2, \textit{relu}2\_2, \textit{relu}3\_2 and \textit{relu}4\_2 as the style layers.
We set the weight for each loss as: 1e5 for content, 2 for style, 1e-7 for spatial regularization, 10 for optical flow, and 100 for shift.
The downsampling factor $K$ for the transformer network \cite{johnson2016perceptual} is $4$.
Shifts are uniformly sampled from $[1,K-1]$ for every training frame.

We follow the same procedure of computing the temporal error as in \cite{huang2017real} to evaluate the consistency between consecutive frames:
\begin{align}
& E _ {temporal} = \nonumber\\
  & \sqrt { \frac {1} { (T-1) \times M } \sum _ { t = 1 } ^ { T - 1 } \sum _ { m = 1 } ^ { M } \mathbf { c } _ { m } \left( \hat {s } _ { m } ^ { t } - f \left( \hat { s } _ { m } ^ { t + 1 } \right) \right) ^ { 2 } },
  \nonumber
\end{align}

where $N$ is the number of all pixels (width $\times$ hight $\times$ channel) and $T$ represents the length of the sequence. $f$ wraps the stylized frame $t+1$ back to $t$ based on the ground truth optical flow provided in the \textit{Sintel} datset.
Fig. 3 in the main paper shows a sample temporal error map for two consecutive frames.

We train all the three methods for $40,000$ steps on the collected Videvo dataset with an Nvidia GTX 1080 Ti. The batch size is 1.
The training time for of \textit{FF}, \textit{FF+flow} and \textit {Ours} are 3.27, 3.33 and 5.18 hours respectively.
Note that it takes approximately 3 hours before training to compute the optical flow which is required for the training of the \textit{FF+flow} method, and this method also requires sequential training data while \textit{Ours} does not.

\subsection{Training details of Carla benchmark evalution}
We use the goal-directed navigation benchmark \cite{dosovitskiy2017carla} in \textit{Carla} simulator.
We deploy all experiments in Town 1 and test under the testing weather condition.
There are four tasks in the benchmark including \textit{Straight}, \textit{One turn}, \textit{Navigation} and \textit{Navigation with dynamic obstacles}.
Each of the tasks is carried out over 25 episodes.
Each episode has a preset starting and goal location.
The agent needs to reach the goal within a certain time budget to achieve a successful episode.
The time budget is defined by the time needed to reach the goal when travelling along the optimal path within 10 km/h.
The optimal path to finish all $25\times4$ episodes in the benchmark is around 53 km.

% \hl{training results comparable}

All of the training of the policies and the adaptation models are implemented with Pytorch and deployed with a single Nvidia 1080Ti GPU.
Images provided in the \textit{Carla} dataset are of size $88\times200$.
We train our visual control policy following the branched structure of condition imitation learning \cite{Codevilla2018}.
The speed of the car is also taken as the input.
Four differnt branches corresponds to four differnt high level commands (\textit{straight}, \textit{left}, \textit{right}, \textit{follow line}) provided by the global path planner.
Each of the branches will output three values indicating the steering angle, the acceleration and the brake respectively.
The embedding of the image is also used to predict the speed of the car as an auxiliary task.
The same data augmentation methods as in \cite{Codevilla2018} are incorporated including contrast variations, brightness and tone variations, adding Gaussian blur, Gaussian noise and salt-and-pepper noise, and masking out a random set of rectangles in the image.
The batch size for training is 1000. Our implementation code for this part is public\footnote{https://github.com/onlytailei/carla\_cil\_pytorch}.
\begin{table}[h]
\centering
\begin{tabular}{ccccc}
\hline
\multicolumn{1}{l}{} & \multicolumn{1}{c}{daytime} & \multicolumn{1}{c}{daytime} & \multicolumn{1}{c}{clear} & \multicolumn{1}{c}{daytime} \\
                     &                             & after rain                  & sunset                    & hard rain                   \\ \hline
Training                & 853                         & 840                         & 715                       & 816                         \\ \hline
Evaluation                 & 99                          & 99                          & 84                        & 93                          \\ \hline
\end{tabular}
\caption{Sequence data distribution under the four different weathers of the original \textit{Carla} dataset. Each of the sequence consists of 200 frames.}
\label{carla_dataset}
\end{table}

The original \text{Carla} dataset consists of 3289 sequences for training and 374 sequences for evaluating where each sequence includes 200 frames. We separate them based on the four weather conditions as shown in Table \ref{carla_dataset}.

We train all of the policies for 90 epochs with Adam and an initial learning rate of 0.0002.
The learning rate is reduced by half every ten epochs.
The training for each of the three \textit{Single-Domain} policies takes around 5 hours under its corresponding training weather condition.
The training of the \textit{Multi-Domain} policy takes almost 16 hours since it uses all of three training weather conditions as described in Section IV-B. of the main paper.
The evaluation dataset is used to choose the best model after each epoch.
We randomly choose 30 sequences from the evaluation data under each of the three training weather conditions as the evaluation data for \textit{Multi-Domain}. Our policy shows comparable quality compared with the original implementation \cite{dosovitskiy2017carla} in training conditions as reported in Table II of our main paper.

Three transfer models are trained to translate images from the testing weather condition (\textit{daytime hard rain}) to each of the three training conditions for both \textit{CycleGan} and \textit{VR-Goggles}.
We follow the default settings of official CycleGAN code\footnote{https://github.com/junyanz/pytorch-CycleGAN-and-pix2pix}.
We do not conduct any resizing or cropping during training.
The learning rate is 0.0002 for the first
100 and decayed to 0 for the next 100 epochs.
The weight of the shift loss is 1000.
The domain adaptation takes almost the same time for both \textit{CycleGAN} and \textit{VR-Goggles}, which is almost 15 hours.
The last models for all of the setups are used for the benchmark testing.
In fact, the visual quality of the generated image is quite stable after 50 epochs as shown in Figure \ref{fig:epoch_check}, and we don't really need to train the model for 15 hours for applications. However, to compare with the original CycleGAn fairly, we follow their settings for the account of training epoch \cite{zhu2017unpaired}. For the experiments in the real world (Section IV.C. of the main paper), we train \textit{CycleGAN} and \textit{VR-Goggles} for 50 epochs.

\begin{figure}[t]
    \centering
    \begin{subfigure}{0.48\columnwidth}
    \centering
        \includegraphics[width=\columnwidth]{imgs/stage_compare/raw}
        \caption{Input}
        \label{fig:input}
    \end{subfigure}
    \begin{subfigure}{0.48\columnwidth}
    \centering
        \includegraphics[width=\columnwidth]{imgs/stage_compare/5}
        \caption{5 epochs}
        \label{fig:out5}
    \end{subfigure}
    \begin{subfigure}{0.48\columnwidth}
    \centering
        \includegraphics[width=\columnwidth]{imgs/stage_compare/50}
        \caption{50 epochs}
        \label{fig:out50}
    \end{subfigure}
    \begin{subfigure}{0.48\columnwidth}
    \centering
        \includegraphics[width=\columnwidth]{imgs/stage_compare/100}
        \caption{100 epochs}
        \label{fig:out100}
    \end{subfigure}
    \begin{subfigure}{0.48\columnwidth}
    \centering
        \includegraphics[width=\columnwidth]{imgs/stage_compare/150}
        \caption{150 epochs}
        \label{fig:out150}
    \end{subfigure}
    \begin{subfigure}{0.48\columnwidth}
    \centering
        \includegraphics[width=\columnwidth]{imgs/stage_compare/200}
        \caption{200 epochs}
        \label{fig:out200}
    \end{subfigure}
    \caption{
    The effects of \textit{VR-Goggles} transfer model training at different training stages.
    After 50 epochs, the output of the transfer model is quite stable.
    }
    \label{fig:epoch_check}
  \vspace{-0.05in}
\end{figure}

An interesting point in Table II of the main paper is that testing result under the \textit{Multi-Domain} policy is better than in training condition for the \textit{Straight} task.
It is also the case in the results presented in the original \textit{Carla} benchmark tests \cite{dosovitskiy2017carla}.
