# Supplementary material for: VR-Goggles for Robots: Real-to-sim Domain Adaptation for Visual Control
Source: arXiv:1802.00265 source file (2019-01-16)
Supplement: Supplementary file 4 [file appendix1.tex]

\subsection{Validating Shift Loss: Additional Materials}
\label{apd:shift-loss}

\begin{figure}[!h]
    \centering
        \includegraphics[width=\columnwidth]{imgs/shift_sequence/shift_sequence}
    % \vspace{-0.1in}
    \caption{
    % \textit{Error maps} between generated stylizations for subsequence input frames.
    % $\nth{1}$ \textit{row}: input frames; $\nth{2}\sim\nth{4}$ \textit{row}: error maps (with the corresponding stylizations shown on top) of outputs from \textit{FF}, \textit{FF+flow} and \textit{Ours}.
    % We here choose a very challenging style (\textit{mosaic}) for temporal consistence, as it contains many fine details that tiny tiles are laid over the original image in the final stylizations.
    % Yet, \textit{Ours} is achieving a very high consistence, which can be observed more clearly in our attached video \hl{video link}.}
    \textit{Temporal error maps} between generated stylizations for subsequence input frames.
    $\nth{1}$ \textit{row}: input frames; $\nth{2}\sim\nth{4}$ \textit{row}: temporal error maps (with the corresponding stylizations shown on top) of outputs from \textit{FF}, \textit{FF+flow}, and \textit{Ours}.
    We here choose a very challenging style (\textit{mosaic}) for temporal consistency, as it contains many fine details, with tiny tiles laid over the original image in the final stylizations.
    Yet, \textit{Ours} achieves very high consistency.}%, which can be observed more clearly in our attached video \hl{video link}.}
   \label{fig:shift-sequence}
\end{figure}

We conduct additional experiments for evaluating the consistency of the stylized sequential input frames. In Fig. \ref{fig:shift-sequence}, we show the \textit{temporal error maps}, the same metric as in \cite{huang2017real}, of two stylized consecutive frames for each method.
\textit{Ours} (bottom row) achieves the highest temporal consistency. The more high-resolution stylized sequences are available in the video.

Further details for all \textit{shift loss} experiments:
We do not compare with \cite{ruder2017artistic} as they require optical flow as input during testing,
which is relatively expensive for our target application of real-time robotics control.
